# Supplementary material for: Phosphorene nanoribbons
Source: arXiv:1404.5115 source file (2014-08-29)
Supplement: Supplementary file 1 [file SI.pdf]

# Phosphorene nanoribbons: Supporting Information

A. Carvalho[1], A. S. Rodin[2] A. H. Castro Neto[1,2]
[1] *Graphene Research Centre and Department of Physics, National University of Singapore, 117542, Singapore*
[2] *Boston University, 590 Commonwealth Ave., Boston MA 02215, USA*

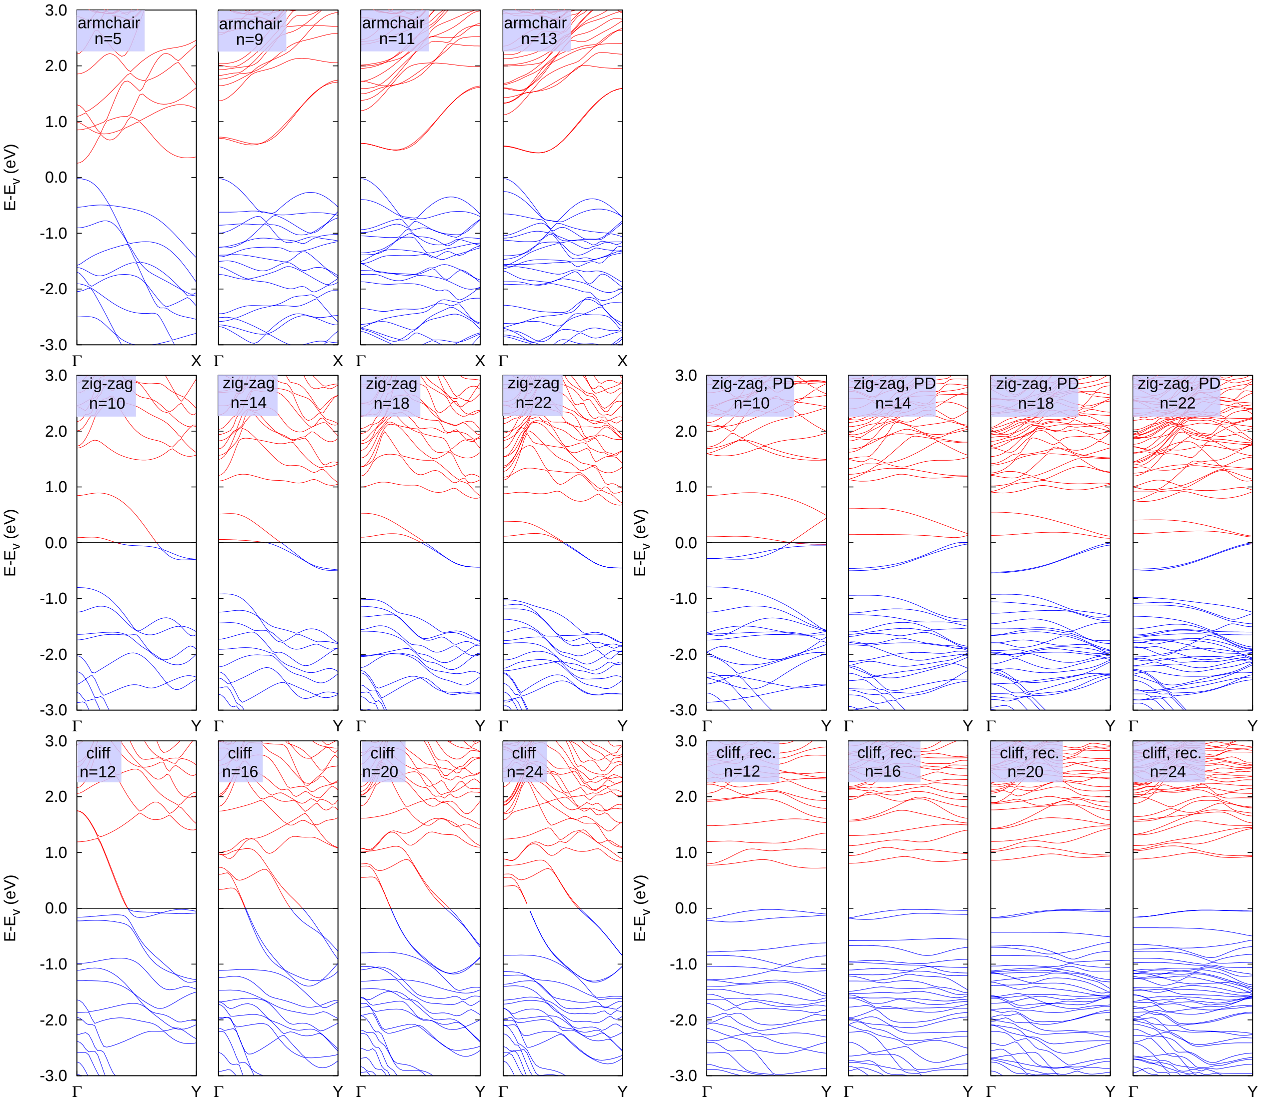


Figure 1: (Color online) Bandstructures of phosphorene nanoribbons. Left: nanoribbons maintaining the original periodicity; Right: Bandstructure following structural relaxation with unit-cell doubling. The zero of the energy scale is set to the valence band top or to the Fermi level (for the metals).

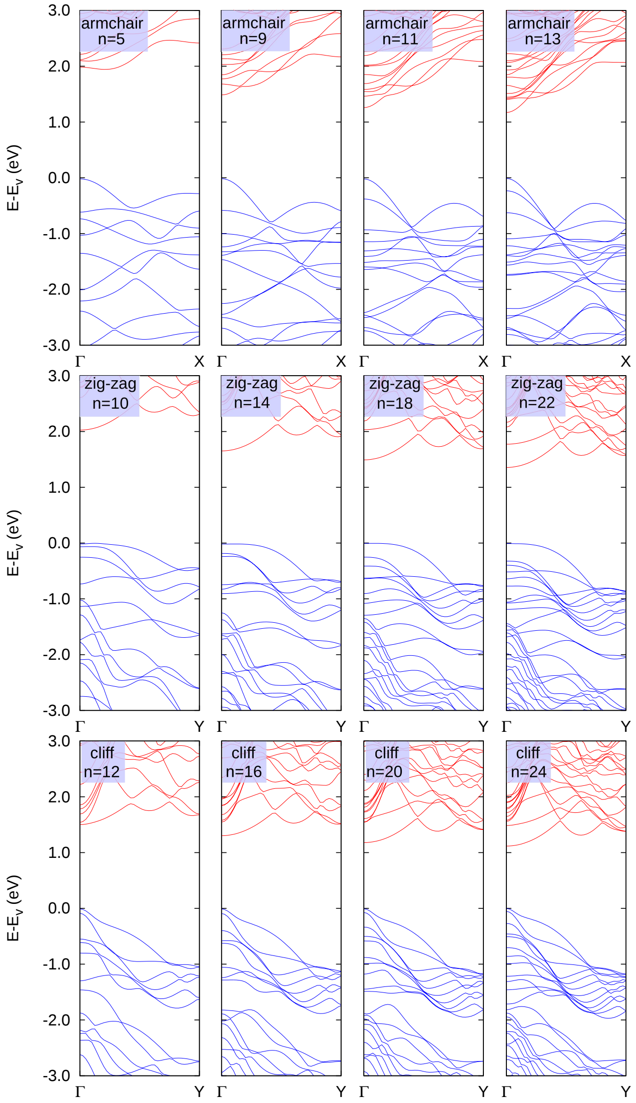


Figure 2: (Color online) Bandstructures of hydrogen-passivated phosphorene nanoribbons. The zero of the energy scale is set to the valence band top or to the Fermi level (for the metals).
